# Supplementary material for: Enhancing Fine-Grained Visual Recognition in the Low-Data Regime Through Feature Magnitude Regularization
Source: arXiv:2409.01672 source file (2024-09-07)
Supplement: Supplementary file 1 [file X_suppl.tex]

\clearpage
\setcounter{page}{1}
\maketitlesupplementary

\section{CARS Images}

\begin{figure}
\centering
    \includegraphics[width=3in]{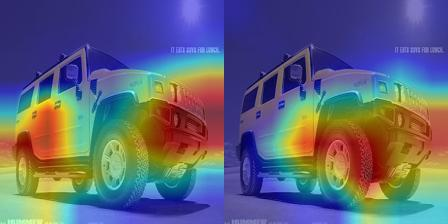}
    \caption{CARS 000084.jpg}
\end{figure}

\begin{figure}
\centering
    \includegraphics[width=3in]{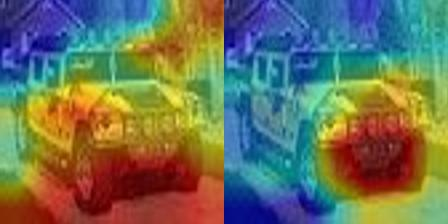}
    \caption{CARS 000089.jpg}
\end{figure}

\begin{figure}
\centering
    \includegraphics[width=3in]{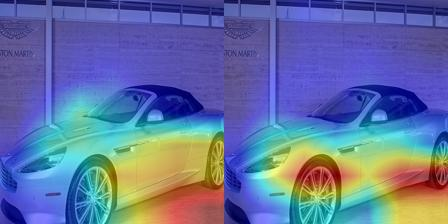}
    \caption{CARS 000778.jpg}
\end{figure}

\begin{figure}
\centering
    \includegraphics[width=3in]{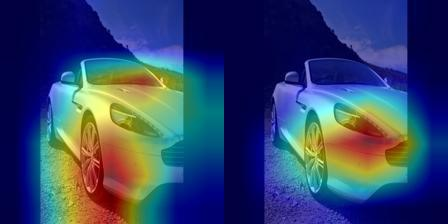}
    \caption{CARS 000790.jpg}
\end{figure}

\begin{figure}
\centering
    \includegraphics[width=3in]{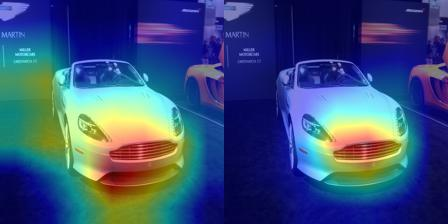}
    \caption{CARS 000793.jpg}
\end{figure}

\begin{figure}
\centering
    \includegraphics[width=3in]{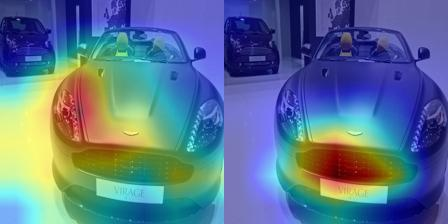}
    \caption{CARS 000794.jpg}
\end{figure}

\begin{figure}
\centering
    \includegraphics[width=3in]{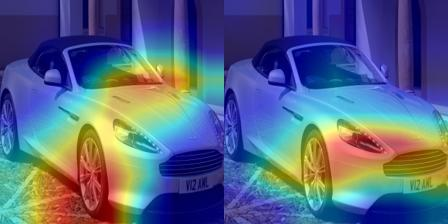}
    \caption{CARS 000795.jpg}
\end{figure}

\begin{figure}
\centering
    \includegraphics[width=3in]{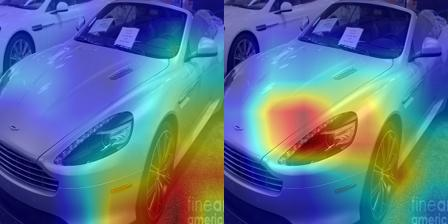}
    \caption{CARS 000796.jpg}
\end{figure}

\begin{figure}
\centering
    \includegraphics[width=3in]{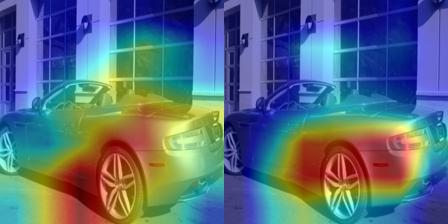}
    \caption{CARS 000797.jpg}
\end{figure}

\begin{figure}
\centering
    \includegraphics[width=3in]{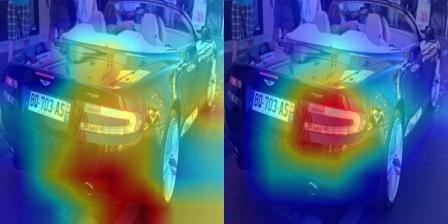}
    \caption{CARS 000805.jpg}
\end{figure}

\begin{figure}
\centering
    \includegraphics[width=3in]{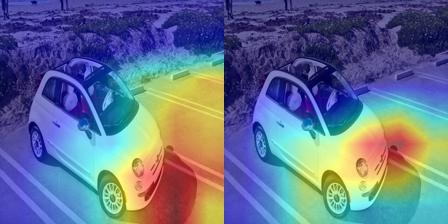}
    \caption{CARS 008146.jpg}
\end{figure}

\section{FGVC AC Images}

\begin{figure}
\centering
    \includegraphics[width=3in]{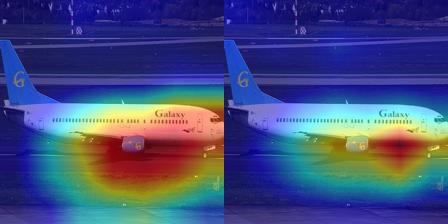}
    \caption{FGVCAC 0076843.jpg}
\end{figure}

\begin{figure}
\centering
    \includegraphics[width=3in]{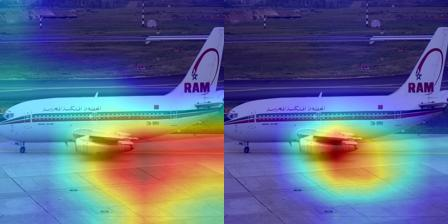}
    \caption{FGVCAC 0127648.jpg}
\end{figure}

\begin{figure}
\centering
    \includegraphics[width=3in]{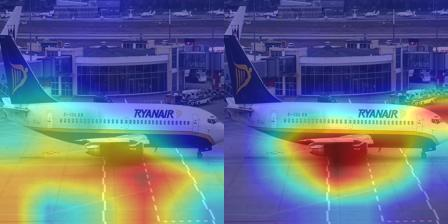}
    \caption{FGVCAC 0225218.jpg}
\end{figure}

\begin{figure}
\centering
    \includegraphics[width=3in]{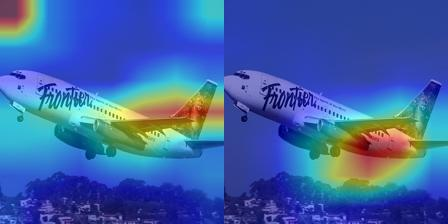}
    \caption{FGVCAC 0227058.jpg}
\end{figure}

\begin{figure}
\centering
    \includegraphics[width=3in]{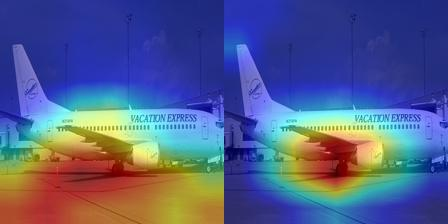}
    \caption{FGVCAC 0357873.jpg}
\end{figure}

\begin{figure}
\centering
    \includegraphics[width=3in]{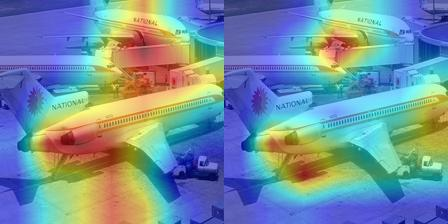}
    \caption{FGVCAC 0538261.jpg}
\end{figure}

\begin{figure}
\centering
    \includegraphics[width=3in]{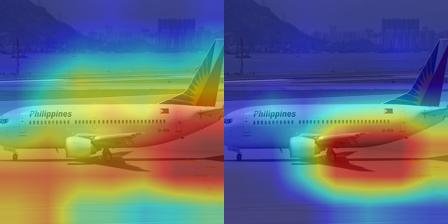}
    \caption{FGVCAC 0681541.jpg}
\end{figure}

\begin{figure}
\centering
    \includegraphics[width=3in]{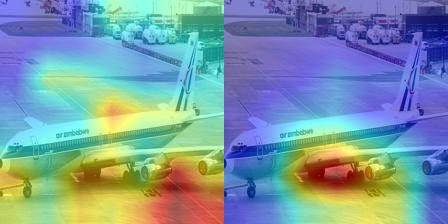}
    \caption{FGVCAC 0691159.jpg}
\end{figure}

\section{CUB200 Images}

\begin{figure}
\centering
    \includegraphics[width=3in]{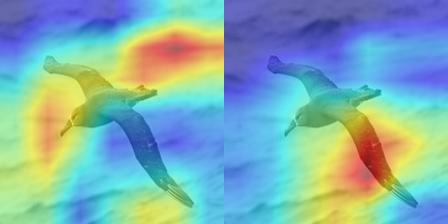}
    \caption{CUB200 Black\_Footed\_Albatross\_0001\_796111.jpg}
\end{figure}

\begin{figure}
\centering
    \includegraphics[width=3in]{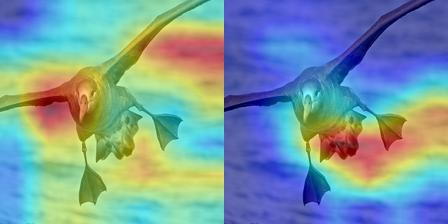}
    \caption{CUB200 Black\_Footed\_Albatross\_0005\_796090.jpg}
\end{figure}

\begin{figure}
\centering
    \includegraphics[width=3in]{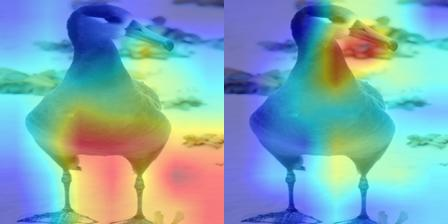}
    \caption{CUB200 Black\_Footed\_Albatross\_0049\_796063.jpg}
\end{figure}

\begin{figure}
\centering
    \includegraphics[width=3in]{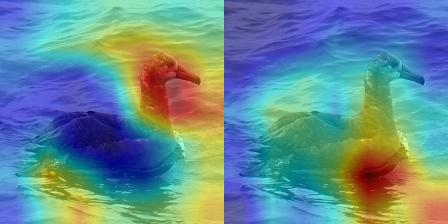}
    \caption{CUB200 Black\_Footed\_Albatross\_0076\_417.jpg}
\end{figure}

\begin{figure}
\centering
    \includegraphics[width=3in]{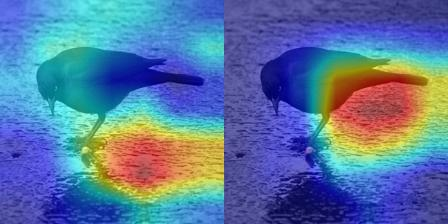}
    \caption{CUB200 Brewer\_Blackbird\_0009\_2616.jpg}
\end{figure}

\begin{figure}
\centering
    \includegraphics[width=3in]{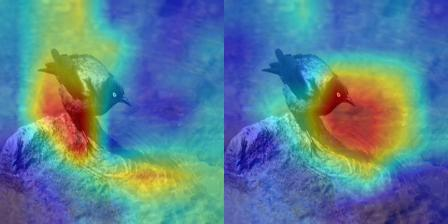}
    \caption{CUB200 Brewer\_Blackbird\_0012\_2691.jpg}
\end{figure}

\begin{figure}
\centering
    \includegraphics[width=3in]{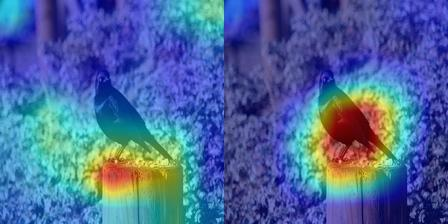}
    \caption{CUB200 Brewer\_Blackbird\_0017\_2668.jpg}
\end{figure}

\begin{figure}
\centering
    \includegraphics[width=3in]{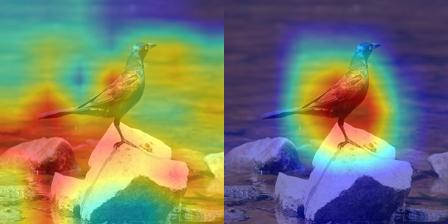}
    \caption{CUB200 Brewer\_Blackbird\_0041\_2653.jpg}
\end{figure}

\begin{figure}
\centering
    \includegraphics[width=3in]{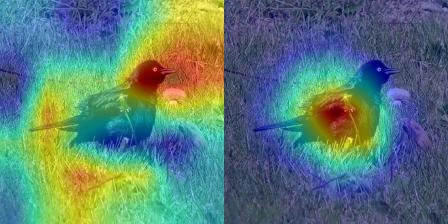}
    \caption{CUB200 Brewer\_Blackbird\_0054\_2631.jpg}
\end{figure}

\section{iNaturalist Images}

\begin{figure}
\centering
    \includegraphics[width=3in]{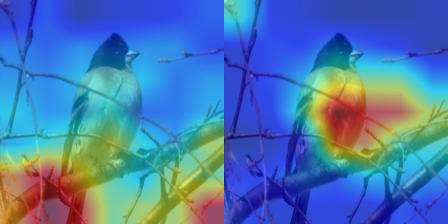}
    \caption{iNaturalist 0aa6d98f-9fc5-4a30-aef4-a54d555c2311.jpg}
\end{figure}

\begin{figure}
\centering
    \includegraphics[width=3in]{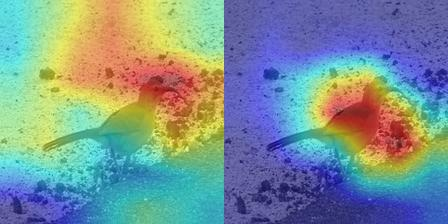}
    \caption{iNaturalist 0c8940c9-59c9-4f09-a005-f6e6868392c4.jpg}
\end{figure}

\begin{figure}
\centering
    \includegraphics[width=3in]{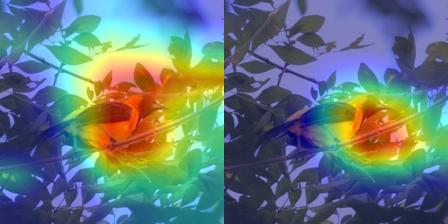}
    \caption{iNaturalist 1aef2ce9-3a68-4583-be8d-3855146f95ad.jpg}
\end{figure}

\begin{figure}
\centering
    \includegraphics[width=3in]{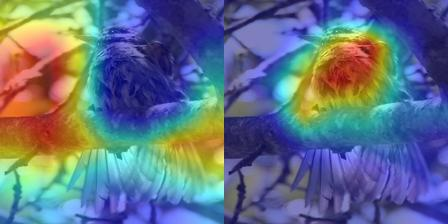}
    \caption{iNaturalist 2a7273f5-9c63-4460-8898-e71289a066bd.jpg}
\end{figure}

\begin{figure}
\centering
    \includegraphics[width=3in]{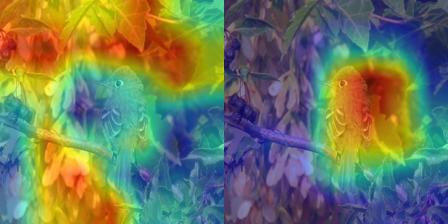}
    \caption{iNaturalist 2c3719a7-87f7-49d9-80df-396885ce3e55.jpg}
\end{figure}

\begin{figure}
\centering
    \includegraphics[width=3in]{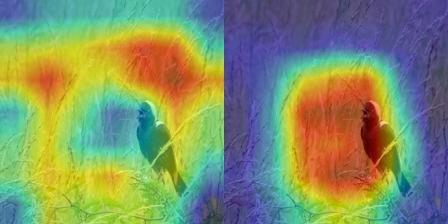}
    \caption{iNaturalist 2deea3bb-b4a9-4363-800f-762f5b3c27df.jpg}
\end{figure}

\begin{figure}
\centering
    \includegraphics[width=3in]{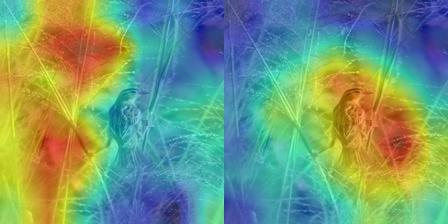}
    \caption{iNaturalist 5a6e5396-c2a6-4967-8734-bac66e921124.jpg}
\end{figure}

\begin{figure}
\centering
    \includegraphics[width=3in]{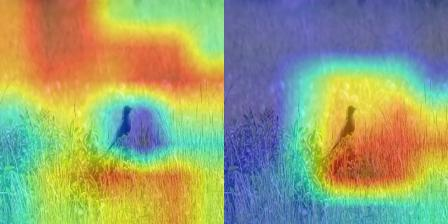}
    \caption{iNaturalist 8f94c9b6-a65d-45a6-b2e3-fc48f50b80c5.jpg}
\end{figure}
